# Supplementary material for: The 2010 Interim Report of the Long-Baseline Neutrino Experiment Collaboration Physics Working Groups
Source: arXiv:1110.6249 source file (2011-10-27)
Supplement: Supplementary file 1 [file Appendix.tex]

%%%%%%%%%%%%%%%%%%%%%%%%%%%%%%%%%%%%%%%%%%%%%%%%%%%%%%%%%%%%%%%%%%%%%%%%%%%%%%%%%%%%%%%%%%%%%%%%%%%%%%%%%%%
%% Version 0.0 7/15/10 RJW Template/outline
%% Filename:    Appendix.tex
%% Description: Appendices if needed.
%% Primary author(s): Bob Wilson
%  Updates:
%   Version 1.0 .......
%
%%%%%%%%%%%%%%%%%%%%%%%%%%%%%%%%%%%%%%%%%%%%%%%%%%%%%%%%%%%%%%%%%%%%%%%%%%%%%%%%%%%%%%%%%%%%%%%%%%%%%%%%%%%
\appendix
\section{And more}\label{appdx1}

\vfill\eject
